# Supplementary material for: Enhanced Meta Reinforcement Learning using Demonstrations in Sparse Reward Environments
Source: arXiv:2209.13048 source file (2022-09-26)
Supplement: Supplementary file 2 [file appendix_gmps_si.tex]

\begin{figure*}[!h]
\centering
\begin{subfigure}{\linewidth}
    \centering
    \includegraphics[width=0.6\linewidth,trim=0 0 0 0,clip]{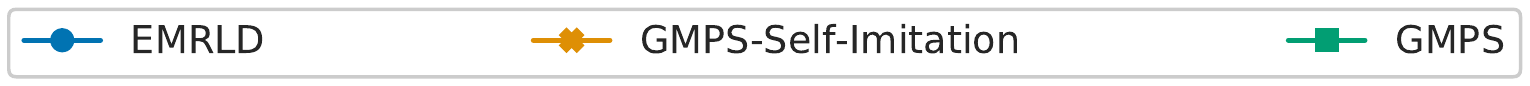}
\end{subfigure}
\vspace{-0.05in}
\begin{subfigure}{\linewidth}
    \centering
    \includegraphics[width=\linewidth]{NeurIPS_2022/sections/figures/appendix/gmps_self_imitation.pdf} %,height=1in
\end{subfigure}
\caption{\textcolor{blue}{Performance of GMPS with Self Imitation in the meta-update step. (a) EMRLD, GMPS-Self-Imitation and GMPS run on Point2D Navigation environment with optimal demonstration data. (b) Zoomed-in view of (a) to clearly show the scale of cumulative reward attained by GMPS-Self-Imitation and GMPS. (c) EMRLD, GMPS-Self-Imitation and GMPS run on Point2D Navigation environment with sub-optimal demonstration data. (d) Zoomed-in view of (c) to clearly show the scale of cumulative reward attained by GMPS-Self-Imitation and GMPS.}}
\label{fig:gmps_si}
\end{figure*}
